# Supplementary material for: TTD: Text-Tag Self-Distillation Enhancing Image-Text Alignment in CLIP to Alleviate Single Tag Bias
Source: arXiv:2404.00384 source file (2024-05-21)
Supplement: Supplementary file 1 [file exp_supp_tag_sensi.tex]

\definecolor{pink}{rgb}{0.96,0.82,0.82}

\setlength{\tabcolsep}{1.5pt}
\begin{table}[!tb]
  \caption{\textbf{Sensitivity of scoring methods based on threshold}. 
  % We utilize image and text encoders from TCL~\cite{cha2023learning} for scoring.
  }
  \label{tab:supp_tagacc_thrd}
  \centering
  \resizebox{0.5\textwidth}{!}{
  \begin{tabular}{@{}lccccc@{}}
    \toprule
    Scoring & P & R & F1 & Acc & mAP\\
    \midrule
    \midrule
    $s_{\mathrm{image}}$ (\cref{eq:s_image})        & 92.5 & 28.6 & 43.7 & 79.5 & 83.2 \\ 
    \midrule
    $s_{\mathrm{pixel}}^{\mathrm{ours}}$ (\cref{eq:s_pixel})        & 82.9 & 74.5 & 78.5 & 88.6 & 90.3 \\
    + TTD (Ours)        & 88.3 & 78.0 & 82.8 & 91.0 & 93.7 \\
  \bottomrule
  \end{tabular}
  }
\end{table}
